# Supplementary material for: Enhancing Classifier Conservativeness and Robustness by Polynomiality
Source: arXiv:2203.12693 source file (2022-03-23)
Supplement: Supplementary file 1 [file appendix.tex]

% \appendix
% \section*{Appendices}
% % \begin{appendices}
% \section{Gaussian infinity demonstration}\label{appendix: Gaussian}
% We prove that the posterior $p(y|x)$ will approximate 0 or 1 when c goes to infinity for LDA and QDA with Gaussian assumption:
% \begin{equation}\label{eq: Gaussian infinity_appendix}
% \begin{aligned}
%         &\lim_{c\to\infty} \frac{p(cx|y_i)}{\sum_k p(cx|y_k)}\\
%     =&\lim_{c\to\infty} \frac{\exp(-\frac{(cx-\mu_i)^2}{2\sigma_i^2})}{\sum_k \exp(-\frac{(cx-\mu_k)^2}{2\sigma_k^2})}\\
%     =& \lim_{c\to\infty} \frac{\exp(-\frac{(cx)^2}{2\sigma_i^2} + \frac{\mu_i(cx)}{\sigma_i^2} -\frac{\mu_i^2}{2\sigma_i^2})}
%     {\sum_k\exp(-\frac{(cx)^2}{2\sigma_k^2} + \frac{\mu_k(cx)}{\sigma_k^2} -\frac{\mu_k^2}{2\sigma_k^2})}\\
%     =&\resizebox{0.5\textwidth}{!}{$\lim_{c\to\infty} \frac{1}{\sum_k\exp(\frac{1}{2}(\frac{1}{\sigma_i^2} - \frac{1}{\sigma_k^2})(cx)^2 + (\frac{\mu_k}{\sigma_k^2} - \frac{\mu_i}{\sigma_i^2})(cx) -\frac{\mu_k^2}{2\sigma_k^2} + \frac{\mu_i^2}{2\sigma_i^2})}$}\\
%     =&\resizebox{0.5\textwidth}{!}{$\lim_{c\to\infty} \frac{1}{\sum_{k, k\neq i}\exp(\frac{1}{2}(\frac{1}{\sigma_i^2} - \frac{1}{\sigma_k^2})(cx)^2 + (\frac{\mu_k}{\sigma_k^2} - \frac{\mu_i}{\sigma_i^2})(cx) -\frac{\mu_k^2}{2\sigma_k^2} + \frac{\mu_i^2}{2\sigma_i^2}) + 1}$}\\
%     =&\resizebox{0.5\textwidth}{!}{$\lim_{c\to\infty}\frac{1}{\sum_{k, k \neq i}\exp((cx)^2(\frac{1}{2}(\frac{1}{\sigma_i^2} -\frac{1}{\sigma_k^2}) +(\frac{\mu_k}{\sigma_k^2} - \frac{\mu_i}{\sigma_i^2})\frac{1}{cx}) - \frac{\mu_k^2}{2\sigma_k^2} + \frac{\mu_i^2}{2\sigma_i^2}) + 1}$}
% \end{aligned}
% \end{equation}

% In the QDA setting, variances of different classes are considered, so the posterior of a sample in the infinity is determined by the variance only:
% \begin{equation}
% \lim_{c\to\infty} \frac{p(cx|y_i)}{\sum_k p(cx|y_k)}=\lim_{c\to\infty}\frac{1}{\sum_{k, k \neq i}\exp((cx)^2(\frac{1}{\sigma_i^2} -\frac{1}{\sigma_k^2})) + 1}
% \end{equation}

% In the setting of LDA, the variance is ignored thus the posterior in the infinity is decided by the mean:
% \begin{equation}
% \lim_{c\to\infty} \frac{p(cx|y_i)}{\sum_k p(cx|y_k)}=\lim_{c\to\infty}\frac{1}{\sum_{k, k \neq i}\exp(cx(\mu_k - \mu_i) + 1}
% \end{equation}


% \section{Polynomial infinity demonstration}\label{appendix: polynomial}
% We need: $\lim_{c\to\infty}\frac{p(cx|y_k)}{p(cx|y_i)} \to 1$ for a conservative prediction.
% If we assume polynomial class conditional distributions and the highest power of $p(x|y_i), p(x|y_j)$ is $a, b$ respectively and if we want:
% \begin{equation}\label{eq: power of pdf}
% \begin{aligned}
%     & \lim_{c\to\infty}\frac{(c\|x\|)^a}{(c\|x\|)^b} \to 1\\
%   =& \lim_{c\to\infty}(c\|x\|)^{a-b} \to 1\\
%   & a = b
% \end{aligned}
% \end{equation}
% The highest power of the polynomial class conditional distribution should be the same for all the classes to guarantee a conservative prediction. Student's $t$-distribution is therefore feasible. 
